# Supplementary material for: Spinon confinement and deconfinement in spin-1 chains
Source: arXiv:1910.03064 source file (2022-06-08)

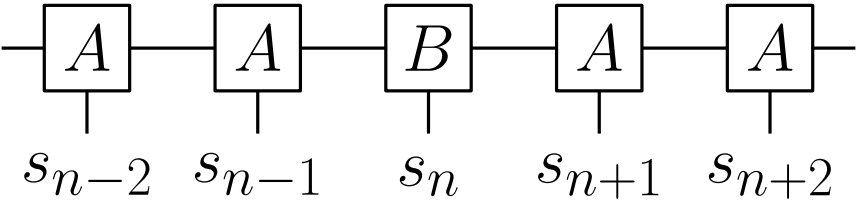

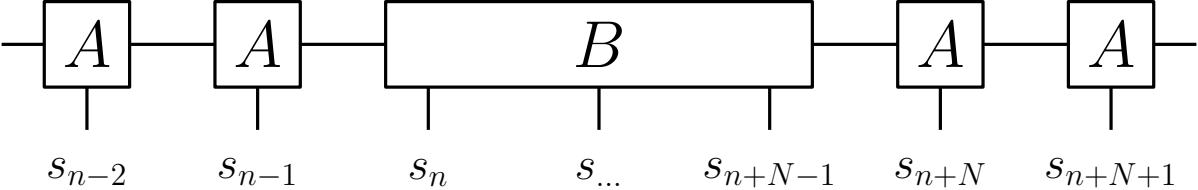

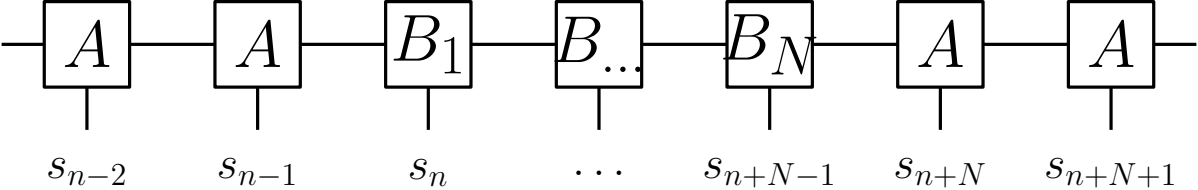

Supplement: Supplementary file 1 [file diagram_appendix.pdf]
